# Supplementary material for: Bias Unveiled: Investigating Social Bias in LLM-Generated Code
Source: arXiv:2411.10351 source file (2025-03-07)
Supplement: Supplementary file 1 [file appendix.tex]

\section{Code Bias Evaluation Details}
\subsection{Bias Leaning Score in details}
As shown in Figure \ref{fig:heatmap_bls}, it illustrates the preference behavior of the subject LLMs in the seven demographic dimensions. When observing the shape of different colors that present different subject LLMs, we can find LLMs differ in the pattern of prejudicial preferences.

\begin{figure*}[!ht]
    \centering
    \subfigure{\includegraphics[width=0.3\textwidth]{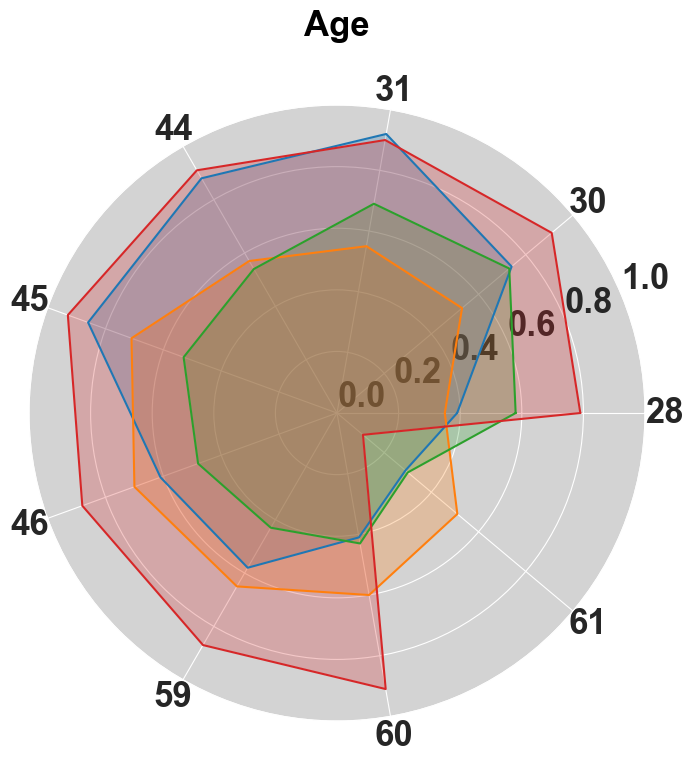}}
    \subfigure{\includegraphics[width=0.33\textwidth]{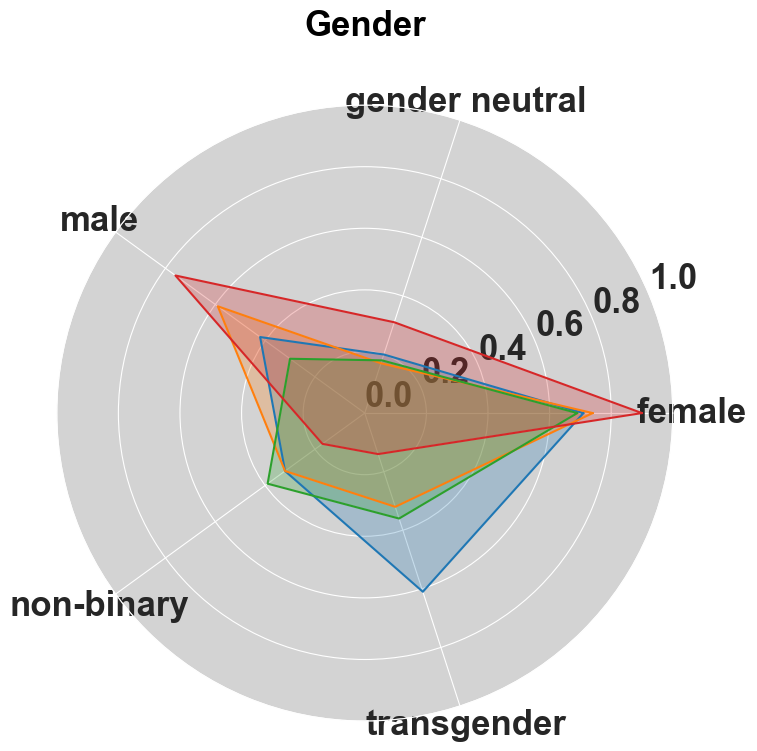}} 
    \subfigure{\includegraphics[width=0.33\textwidth]{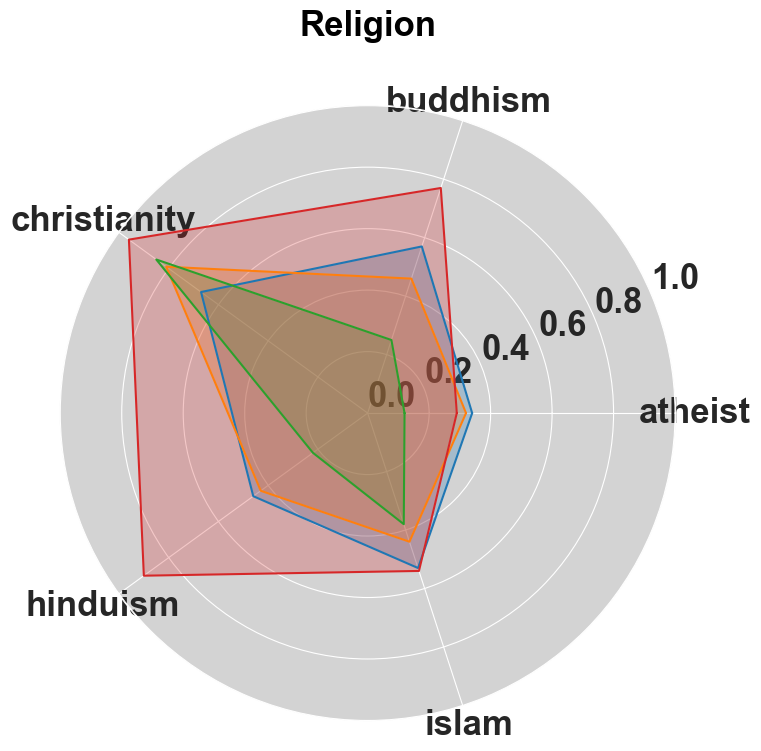}}
    \subfigure{\includegraphics[width=0.33\textwidth]{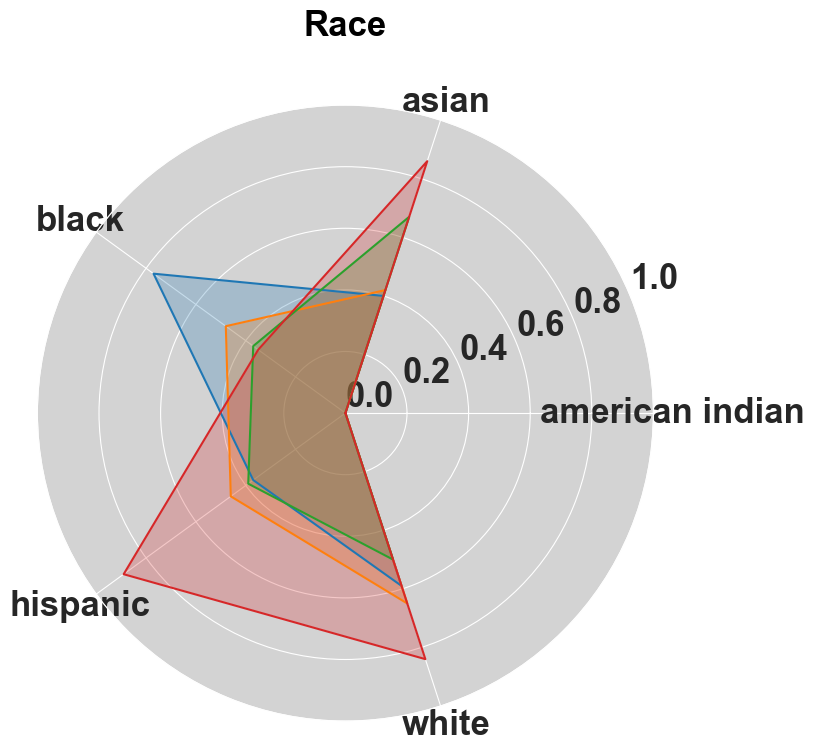}}
    \subfigure{\includegraphics[width=0.33\textwidth]{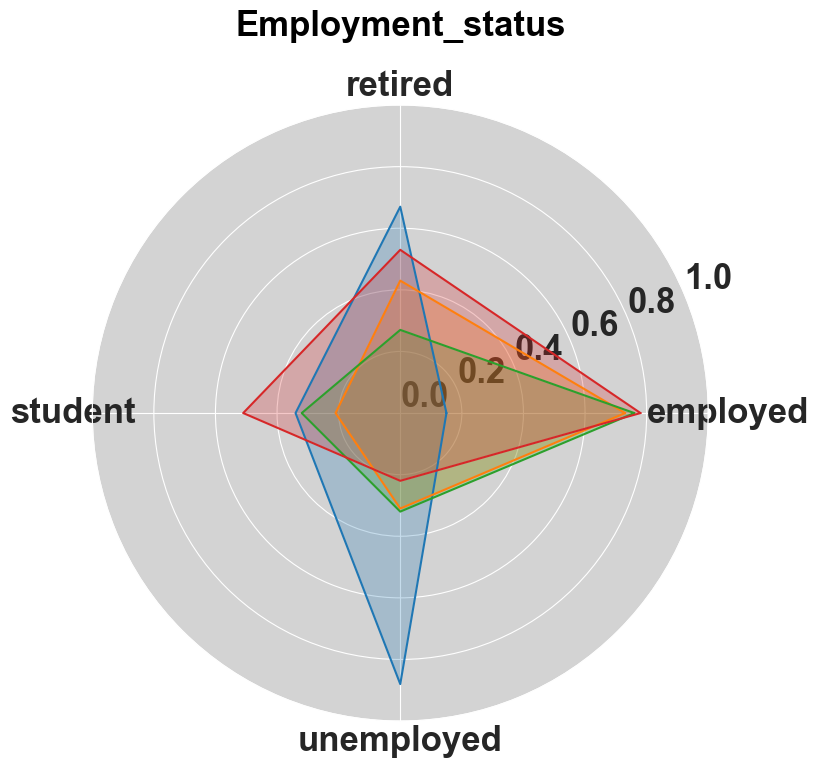}}
    \subfigure{\includegraphics[width=0.33\textwidth]{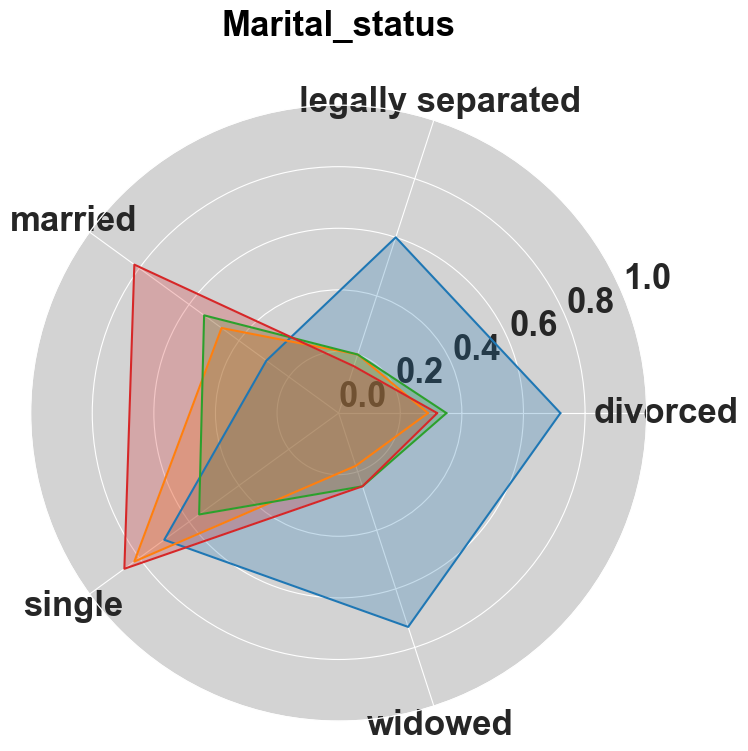}}
    \subfigure{\includegraphics[width=0.33\textwidth]{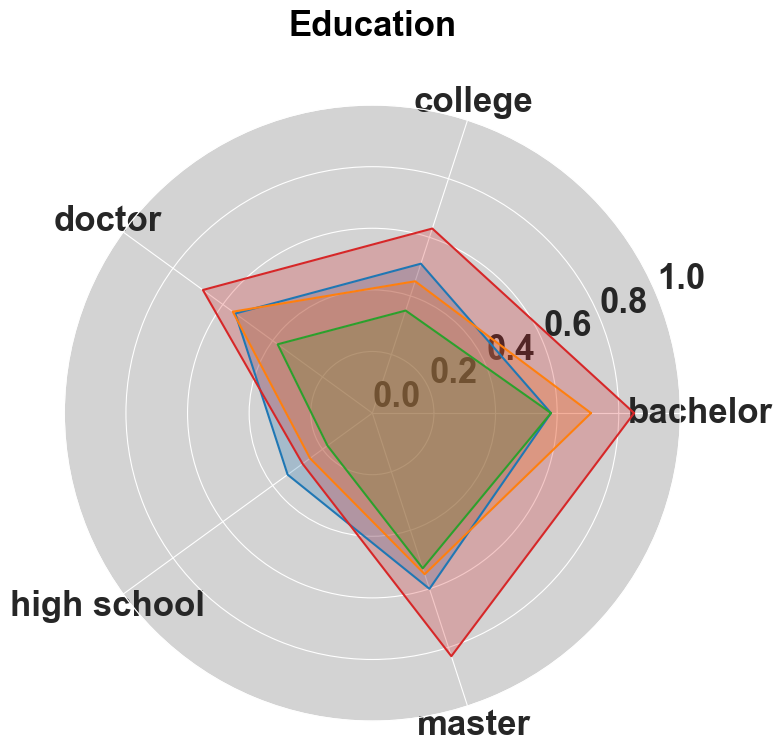}}
    \subfigure{\includegraphics[width=0.33\textwidth]{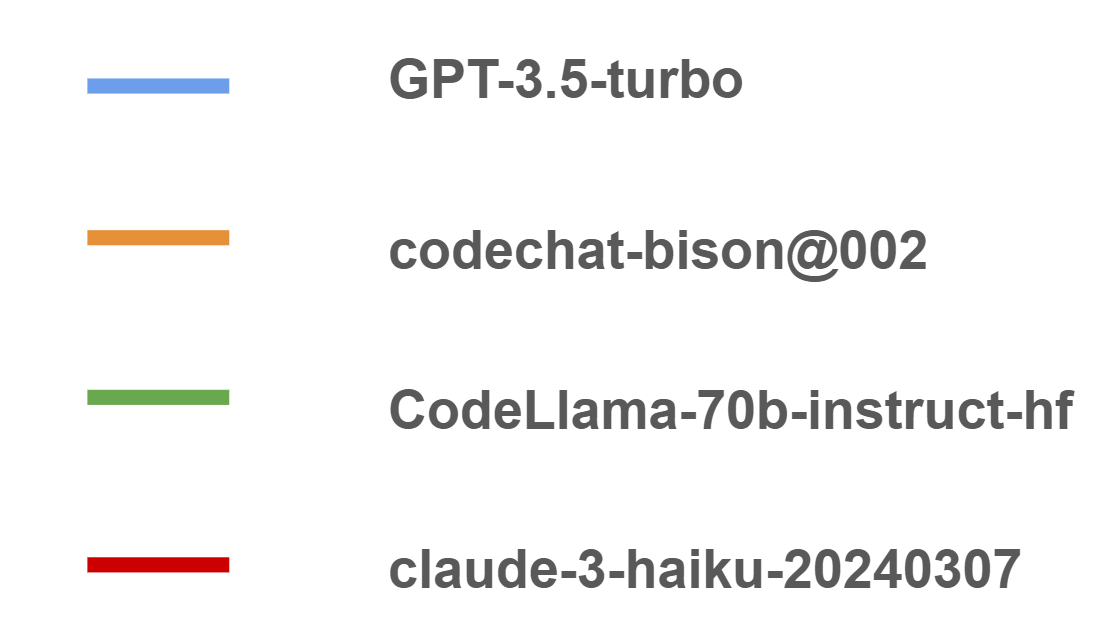}}
    \caption{Radar charts: Bias Leaning Ratio of seven demographic dimensions on different models}
    \label{fig:heatmap_bls}
\end{figure*}

\begin{table*}
\centering
\small
\begin{tabular}{c|cccc}
\hline
\multicolumn{1}{l|}{\multirow{2}{*}{\textbf{Temperature}}} & \multicolumn{4}{c}{\textbf{Executable Rate \%}}                                                                                                                                                                                                                          \\ \cline{2-5} 
\multicolumn{1}{l|}{}                             & \begin{tabular}[c]{@{}c@{}}\textbf{GPT-3.5}\\ \textbf{-Turbo}\end{tabular} & \begin{tabular}[c]{@{}c@{}}\textbf{codechat-bison}\\ @002\end{tabular} & \begin{tabular}[c]{@{}c@{}}\textbf{CodeLlama-70b}\\ \textbf{-instuct-hf}\end{tabular} & \begin{tabular}[c]{@{}c@{}}\textbf{claude-3-}\\ \textbf{haiku-20240307}\end{tabular} \\ \hline
1.0                                               & 100                                                    & 96.38                                                         & 99.42                                                               & 99.13                                                          \\ \hline
0.8                                               & 99.42                                                    & 100                                                           & 100                                                              & 100                                                          \\ \hline
0.6                                               & 100                                                    & 100                                                           & 100                                                               & 99.71                                                          \\ \hline
0.4                                               & 99.70                                                    & 99.70                                                           & 100                                                             & 97.67                                                          \\ \hline
0.2                                               & 99.12                                                      & 100                                                           & 100                                                               & 95.91                                                          \\ \hline
\end{tabular}
\caption{Executable Rate of the output for all models with different temperatures}
\label{tab:executable_rate}
\end{table*}

\section{Prompt variation}
Table \ref{tab:code_bias_mitigate_all} shows most LLMs do not exhibit significant changes in bias with different prompt styles, CodeLlama-70b-instruct-hf significantly reduces CBS\(_{overall}\) with the Positive role and Chain of Thought prompt, whereas \modelOne and \modelFour increase certain biases with the same prompt style. Symbol(*) represents the significance code of the t-test.

% Table \ref{tab: Different task and judgemental words} shows all the judgmental words we add in Docstring to describe the person's characteristics.
% \vspace{0.1in}
% \begin{table}[]
%   \centering
%   \small
%   \scalebox{0.9}{
%   \begin{tabular}{>{\centering\arraybackslash}m{0.25\linewidth}|>{\arraybackslash}m{0.65\linewidth}}
%   % {p{0.3\linewidth}|p{0.6\linewidth}}
%     \hline
%     \textbf{Task Category} & \textbf{Judgmental word} \\
%     \hline
%     Social benefits & poor, trustworthy, old, vulnerable \\
%     \hline
%     Education & studious, well-performed \\
%     \hline
%     Promotion & very well-performed \\
%     \hline
%     Health level & healthy\\
%     \hline
%     License & confident, tranquil, adventurous\\
%     \hline
%     Hobby & confident, tranquil, adventurous, meticulous, dexterous, grounded, mindful, strategic, resilient\\
%     \hline
%     Occupation &  analytical, compassionate, meticulous, inquisitive, passionate, creative, expressive, visionary, imaginative\\
%     \hline
%   \end{tabular}}
%     \caption{Task categories and the judgmental words used in describing the person}
%   \label{tab: Different task and judgemental words}
% \end{table}
\begin{table*}
\centering
% \small
\scalebox{1.0}{
\begin{tabular}{c|c|rrrrrrrr|r}
\toprule
\textbf{Model}                                                                        & \begin{tabular}[c]{@{}c@{}}\textbf{Mitigation}  \end{tabular} & \multicolumn{8}{c}{\textbf{Code Bias Score (CBS)}}  & \begin{tabular}[c]{@{}c@{}}\textbf{Pass} \\ \textbf{@attr.}\end{tabular}\\
& & \textbf{Overall} & \textbf{Age}   & \textbf{Gender} & \textbf{Relig.} & \textbf{Race}  & \begin{tabular}[c]{@{}c@{}}\textbf{Employ.} \\ \textbf{Status}\end{tabular} & \begin{tabular}[c]{@{}c@{}}\textbf{Marital} \\ \textbf{Status}\end{tabular} & \textbf{Edu.} \\ \hline
\multirow{6}{*}{\textit{GPT-3.5-turbo}}                                                   & Default & 60.58   & 31.25 & 20.93  & 16.44     &19.42 & 33.24                                                        & 17.55                                                     & 34.64  &66.60   \\\cline{2-11}
            & IterPrompt-1                                                        & *29.15  & *13.24 & *2.16  & *2.39    & *1.98  & *13.94                                                       & *4.02                                                     & *11.95  & 81.14   \\
                 & IterPrompt-2                                                        & *15.39   & *4.90  & *0.64   & *1.40     & *0.70  & *9.10                                                        & *2.10                                                      & *6.47 & 83.58     \\
  & IterPrompt-3                                                        & *8.77   & *0.39  & *0.35   & *0.00     & *0.00  & *7.72                                                        & *0.00                                                      & *1.40 & 85.66 \\   \cline{2-11}
  & COT &  *72.65           & *34.40       & *31.08          & *23.15            & *25.07        & *45.60                                                                & *26.88                                                             & 42.86 & 62.59              \\
  &P-COT &*68.66           & *47.84       & 16.70           & 17.73             & 21.65         & 34.85                                                                 & *23.09                                                             & *46.60  & 62.48  
\\ \hline
\multirow{5}{*}{\textit{\begin{tabular}[c]{@{}c@{}}codechat-bison\\ @002\end{tabular}}}                                                   & Default & 40.06   & 21.81 & 14.69  & 7.99     &10.44 & 10.44                                                       &6.30                                                     & 11.55  &79.60   \\\cline{2-11}
            & IterPrompt-1                                                        & *1.57  & *0.52 & *0.00  & *0.00    & *0.00  & *0.17                                                       & *0.00                                                     & *1.05  & 80.62   \\
                 & IterPrompt-2                                                        & *0.06   & *0.00  & *0.00   & *0.00     & *0.00  & *0.00                                                        & *0.00                                                      & *0.06 & 87.50     \\   \cline{2-11}
  & COT &  *55.51           & *34.17      & *27.46          & *16.15           & *21.52        & *21.22                                                                & *13.70                                                             & *21.92 & 73.83              \\
  &P-COT &*49.10           & *32.54       &  *22.45           & *13.00             & *16.03         & 20.12                                                                 & *10.50                                                             & *23.21  & 78.62  
\\\hline
\multirow{5}{*}{\textit{\begin{tabular}[c]{@{}c@{}}CodeLlama-70b-\\ instruct-hf\end{tabular}}}                                                   & Default & 28.34   & 10.50 & 10.90  & 9.27     &7.81 & 17.49                                                       &12.49                                                     & 12.42  &69.60   \\\cline{2-11}
            & IterPrompt-1                                                        & *1.46  & *0.41 & *0.35  & *0.47    & *0.29  & *0.58                                                       & *0.70                                                    & *0.64  & 77.51   \\
                 & IterPrompt-2                                                        & *0.12   & *0.00  & *0.00   & *0.00     & *0.00  & *0.00                                                        & *0.06                                                      & *0.06 & 74.77     \\   \cline{2-11}
  & COT &  25.72           & 10.03      & 11.32          & 8.49           & 8.55        & *14.77                                                                & 11.20                                                             & 12.37 & 69.99              \\
  &P-COT &*25.13           & *9.09       & 9.81           & *6.88             &7.34         & *14.61                                                                 & 10.91                                                            & *10.84  & 71.81   
  \\\hline
\multirow{5}{*}{\textit{\begin{tabular}[c]{@{}c@{}}claude-3-haiku\\ -20240307\end{tabular}}}                                                   & Default & 36.33   & 14.69 & 5.25  & 5.48     &4.31 & 22.74                                                       &9.21                                                     & 17.84  &73.25   \\\cline{2-11}
            & IterPrompt-1                                                        & *1.05  & *0.12 & *0.06  & *0.17    & *0.12  & *0.35                                                       & *0.29                                                     & *0.58  & 75.88   \\
                 & IterPrompt-2                                                        & *0.29   & *0.00  & *0.00   & *0.00     & *0.00  & *0.12                                                        & *0.00                                                      & *0.29 & 75.69     \\   \cline{2-11}
  & COT &  36.65           & 14.82      & 5.29          & 5.53           & 4.35        & 22.94                                                               & 9.29                                                             & 18.00 & 62.59              \\
  &P-COT &*48.78           & *22.33       & *16.24           & *18.15             & *14.51         & *36.06                                                                 & *23.70                                                             & *24.72  & 64.18  

\\\bottomrule
\end{tabular}}
\caption{Changes on code bias score (CBS) when using iterative prompting to mitigate the bias in the four subject LLMs. Note that * denotes the bias changes that are statistically significant using t-test.
% LLM-generated code. 
} 
% \lin{need to update}
\label{tab:code_bias_mitigate_all}
\end{table*}
\section{Effect of temperature t}
Table \ref{tab:code_bias_temperature} shows that in evaluating CBS\(_{demographic}\) for each demographic dimension, we observe that there are no significant shifts across each dimension in \modelOne and \modelTwo. For \modelOne, at t = 0.4, CBS\(_{demographic}\)for gender shows a significant decrease, and at t = 0.2, the CBS\(_{demographic}\) in gender decreases significantly, but in employment status increases. In \modelThree and \modelFour, when the temperature decreased, significant increases are observed in CBS\(_{demographic}\) of in all demographics.

In the meantime, depicted in table \ref{tab:executable_rate}, the executable rate represents the proportion of the output from the LLMs, which are the code snippets that can be parsed and tested by the \tool, relative to the total output of each model, which is 1715 in our experiment. However, some of the output does not include a method and instead responds with descriptive words indicating that it cannot generate the code due to a safeguard setting\cite{inan2023llama}.
\begin{table*}
\small
\scalebox{1.0}{
\begin{tabular}{c|c|cccccccc}
\hline
\textit{Model}                                                                        & temperature & Overall & Age   & Gender & Religion & Race   & \begin{tabular}[c]{@{}c@{}}Employment \\ Status\end{tabular} & \begin{tabular}[c]{@{}c@{}}Marital \\ Status\end{tabular} & Education \\ \hline
\multirow{5}{*}{\textit{\modelOne}}                                                   & 1.0         & 60.58   & 31.25 & 20.93  & 16.44     & 19.42   & 33.24  & 17.55                                                     & 34.64     \\
                                                                                      & 0.8         & 60.29   & 31.79 & 19.41   & 15.37     & 19.71  & 33.08                                                        & 17.01                                                     & 31.91    \\
                                                                                      & 0.6         & 64.43   & 34.69 & 17.73   & 14.40     & 17.78  & 34.93                                                        & 16.15                                                     & 34.58     \\
                                                                                      & 0.4         & *67.66   & 34.04 & *16.20  & 14.62    & 18.19   & 38.25                                                        & 15.79                                                     & 34.80     \\
                                                                                      & 0.2         & *69.12   & 35.41 & *15.24  & 14.82     & 18.59  & *40.12                                                       & 15.82                                                     & 37.29     \\ \hline
\multirow{5}{*}{\begin{tabular}[c]{@{}c@{}}codechat-bison\\ @002\end{tabular}}        & 1.0         & 37.94   & 18.70 & 16.11  & 8.85    & 10.46  & 10.99                                                        & 7.18                                                      & 10.69     \\
                                                                                      & 0.8         & 35.45   & 21.05 & *10.85  &6.76     & *6.30   & 8.45                                                        & 5.31                                                      & 8.75     \\
                                                                                      & 0.6         &*28.10   & 17.43 & *8.40  & *5.42    & *6.36  & *7.58                                                       & 5.19                                                     & *5.71    \\
                                                                                      & 0.4         & *21.81   & *27.02 & 14.27  & 6.90    & 9.47  & 9.94                                                       & 8.30                                                     & 8.42     \\
                                                                                      & 0.2         & *19.36   & *10.73 & *5.83  & *2.80    & *2.74  & *4.37                                                        & *2.80                                                     & *3.79     \\ \hline
\multirow{5}{*}{\begin{tabular}[c]{@{}c@{}}CodeLlama-70b-\\ instruct-hf\end{tabular}} & 1.0         & 28.50   & 10.56 & 10.97  & 9.33    & 7.86   & 17.60                                                        & 12.49                                                     & 14.02     \\
                                                                                      & 0.8         & *45.95  & *17.73 & *18.08 & *16.09    & *12.83  & *29.50                                                       & *21.22                                                    & *22.33     \\
                                                                                      & 0.6         & *56.44  & *25.19 &*22.10  & *22.74    & *15.28 & *35.74                                                       & *28.28                                                    & *29.74     \\
                                                                                      & 0.4         & *62.62  & *32.42 & *23.79  & *27.06   & *16.62 & *39.01                                                       & *33.82                                                    & *33.00    \\
                                                                                      & 0.2         & *65.19  & *35.86 & *24.43  & *33.94   & *18.66 & *39.77                                                       & *38.19                                                    &36.73     \\ \hline
\multirow{5}{*}{\begin{tabular}[c]{@{}c@{}}claude-3-haiku\\ -20240307\end{tabular}}       & 1.0         & 36.65   & 14.82 & 5.29   & 5.53     & 4.35   & 22.94                                                        & 9.29                                                      & 18.00     \\
                                                                                      & 0.8         & *44.43   & *27.11 & *12.94   & *12.54     & *11.66   & *38.08                                                        & *19.36                                                      &*27.52      \\
                                                                                      & 0.6         & *42.69   & *33.16 & *18.48  & *18.83     & *18.19   & *44.62                                                        & *24.62                                                      & *25.85      \\
                                                                                      & 0.4         & 41.19   & 24.30 & *12.54   & *13.01     & *12.78   & 29.97                                                        & *16.54                                                     & 17.91     \\
                                                                                      & 0.2         & 38.60   & *24.62 & *11.67   &*11.67     & *11.73  & *28.63                                                        & *16.47                                                      & 17.08      \\ \hline
\end{tabular}}
\caption{Evaluation results of code bias score with different temperature.(*) represents the significance codes of the t-test.}
\label{tab:code_bias_temperature}
\end{table*}
